# Supplementary material for: ChameleMon: Shifting Measurement Attention as Network State Changes
Source: arXiv:2301.00615 source file (2023-07-20)
Supplement: Supplementary file 1 [file Appendix.tex]

{\centering \section*{APPENDIX}}

% \presec
% \section{Evaluation Metrics} \postsec
% \label{sec:met}

% \bbb{1) Recall Rate (RR): } The ratio of the number of correctly reported instances to the number of all correct instances. 

% \bbb{2) Precision Rate (PR): } The ratio of the number of correctly reported instances to the number of all reported instances. 

% \bbb{3) $F_1$ Score:} $\frac{2 \times PR \times RR}{PR + RR}$.
