# Supplementary material for: ChameleMon: Shifting Measurement Attention as Network State Changes
Source: arXiv:2301.00615 source file (2023-07-20)
Supplement: Supplementary file 2 [file temp.tex]

\presec \subsection{Shifting Measurement Attention} \postsec
\label{sec:adjust}
%网络状况可以随时发生变化,尤其是硬件故障发生的时候。
Network state could change at any time, especially when switch hardware or link failure occurs.
%
As a result, the memory required for packet loss detection changes as time elapses, and a fixed memory configuration at compile time can hardly adapt to the changeable network condition.
%
%
For example, suppose that the upstream heavy-hitter encoder, the upstream heavy-loss encoder, and the downstream heavy-loss encoder are configured with the same-sized memory that can record at most 500 flows.
%
As time elapses, if the real-time network condition is that there is only 100 victim flows in the network, then 80\% of the memory configured for the heavy-loss encoders is wasted.
%
%
\ykc{Therefore, it is strongly desired to dynamically reconfigure \ykc{the memory for different \sketchname{}es} at run-time, so as to automatically adapt to the real-time network condition.}
%

Aiming at this target, the central controller executes a round of two-phase self-adaptation every time the data plane collection completes.
%
In the first phase, it senses the real-time network condition, including the number and flow size distribution of flows and victim flows, with the collected data structures.
%
In the second phase, based on the sensed condition, it \ykc{properly} reconfigures the memory for \ykc{different \sketchname{}es of upstream and downstream flow encoders}, and thresholds of the flow classifier at runtime.
%
The self-adaptation will not function immediately, but will function in the next measurement window, so as to avoid interference with measuring the current window.
%The feature of dynamic memory configuration at runtime is further discussed in the P4 implementation in Section \ref{sec:dataimpl}.


To \ykc{simplify the analysis of} the changeable network condition, at a high level, we classify the condition into three levels based on the \ykc{degree} of packet losses\ykc{, \ie, the number of victim flows.}
%
Each level is represented by one of the three colors widely used in traffic lights.
%
%
\textit{Green} network condition represents that the packet losses are rare or even eliminated in the network.
%
Under green network condition, the central controller only reserves a small amount of memory for the heavy-loss encoders to cope with the potential small burst of packet losses.
%
As the packet losses gradually increase, the network condition transitions to \textit{yellow} level when the reserved memory cannot record all the victim flows in the network.
%
Under yellow network condition, the central controller configures the heavy-loss encoders with more than the reserved memory to record all the victim flows.
%
As the packet losses further increase, the central controller configures the heavy-loss encoders with more and more memory, until all the memory of the downstream flow encoder runs out, and then the network condition transitions to \textit{red} level.
%
Under red network condition, the central controller and shifts to record all the heavy-losses instead of all the victim flows, and only reserves a small amount of memory for the upstream heavy-hitter encoder to record some heavy-hitter candidates.
%
To maintain visibility to the number and flow size distribution of victim flows, the central controller also reserves a small amount of memory for the light-loss encoders, so as to record a portion of light-losses through sampling.
%

For each condition level, we detail the two phases in the self-adaptation and how it transitions to the other levels.
%

%Here, we only detail the transition to the adjacent levels because the transitions directly from green to red or from red to green is the same as those first undergo the transition to yellow.

\subsubsection{Green network condition:}

\ykc{Under green network condition, there is a fixed memory configuration that $m_{hh}$, $m_{hl}$ and $m_{ll}$ are set to $m^{uf}-m^{res}_{hl}$, $m^{res}_{hl}$, and $0$, respectively;}
%在这个状况下，只有heavyhitter和heavyloss
For each edge switch, the threshold $T_h$ can be set to arbitrary value and $T_l$ is always set to $0$.
%
Note that $T_h$ is a switch-specific value for maximizing the memory utilization considering different edge switches could have different number of flows and flow size distributions, while $T_l$ is a unified value for capturing the \ykc{top-$k$} heavy-losses in the network.
%
Suppose the network condition sensed in the previous round of self-adaptation is green, and now the central controller starts the next round.
%

%
% \begin{itemize}[leftmargin=*,parsep=0pt,itemsep=0pt,topsep=2pt,partopsep=2pt]

%     \item 
    
%     \item 
    
%     \item 
% \end{itemize}
%
\bbb{Sensing real-time network condition:}
First, for each edge switch, the central controller estimates its number of flows and flow size distribution as described in cardinality estimation and flow size distribution estimation ($\S$~\ref{tasks:flow}).
%the central controller
Second, for each edge switch, the central controller obtains its number of heavy-hitter candidates by decoding its upstream heavy-hitter encoder.
%
If the decoding of any upstream heavy-hitter encoder fails, the central controller \textbf{terminates} the sensing.
%
%Otherwise, it estimates the flow size distribution of each edge switch with the flow classifier and the decoded heavy-hitter candidates as described in flow size distribution estimation ($\S$~\ref{tasks:flow}).
%
Third, the central controller obtains the number of victim flows by decoding the delta heavy-loss encoder as described in packet loss detection ($\S$~\ref{tasks:flow}).
%
If the decoding fails, the central controller further estimates the number of victim flows by applying linear-counting to any bucket array of the delta heavy-loss encoder.

\bbb{Reconfiguring memory and thresholds:}
First, if the decoding of any upstream heavy-hitter encoder fails, the central controller turns up the threshold $T_h$ of the edge switch where it is deployed according to its flow size distribution, so as to control the expected load factor\footnote{load factor refers to the ratio of the number of recorded flows to the number of buckets of \sketchname{}. In an ideal scenario, each bucket of \sketchname{} can record an the ID and frequency of an individual flow.} of the upstream heavy-hitter encoder at around 75\%.
%
Note that under the best parameter settings that the number of bucket arrays $d$ is set to $3$, the maximum load factor is around $81.3\% = \frac{1}{1.23}$, and we decide not to purse the maximum rate is to handle 1) the potential increase of heavy-hitter candidates in the current measurement window and 2) the inevitable estimation error in linear-counting.
%
After turning up the threshold $T_h$, the central controller \textbf{terminates} this round of self-adaptation.
%

Second, if the decoding of the delta heavy-loss encoder fails, according to the estimated number of victim flows, the central controller estimates the required memory for controlling the expected load factor of the delta heavy-loss encoder at around 75\%.
%
If the maximum memory that the upstream and downstream encoders can be configured with, \ie, the downstream flow encoder, can cover the required memory, the green network condition transitions to the yellow network condition.
%
In this case, the central controller just expands the upstream and downstream encoders to the required memory.
%
If the maximum memory cannot cover the required memory, the green network condition transitions to the red network condition.
%
In this case, the central controller 1) reconfigures the memory of \ykc{each \sketchname{} of the upstream and downstream flow encoders as described in Section \ref{sec:red}}, 2) sets the unified threshold $T_l$ to a user-defined value, which is the \ykc{maximum/minimum} $T_h$ among all edge switches by default, and 3) sets the sampling rate to control the expected load factor of the delta light-loss encoder at around 75\% 
assuming that every victim flow could be a light-loss.
%
%

After all the memory reconfigurations, for each edge switch, with the number of heavy-hitter candidates and the memory of the upstream heavy-hitter encoder, the central controller further estimates the the expected load factor of the upstream heavy-hitter encoder.
%
if the expected load factor of any upstream heavy-hitter encoder is lower than 60\% or larger than 75\%, the central controller also turns down or up the threshold $T_h$ of the edge switch where it is deployed to approach 75\% load factor.
%

\subsubsection{Yellow network condition:}
Under yellow network condition, the memory configuration is not fixed, that $m_{hh}$ and $m_{hl}$ can vary from $m^{res}_{hh}$ to $m_{uf} - m^{res}_{hl}$ and from $m_{uf} - m^{res}_{hh}$ to $m^{res}_{hl}$, respectively, while $m_{ll}$ is always set to $0$;
%
For each edge switch, the threshold $T_h$ can be set to arbitrary value and $T_l$ is always set to $0$.
%
Suppose the network condition sensed in the last round of self-adaptation is yellow, and now the central controller starts the next round.

\bbb{Sensing real-time network condition:}
The same as that in green network condition.

\bbb{Reconfiguring memory and thresholds:}
Almost the same as that in green network condition.
%
In addition, when no decoding fails and the load factor of the delta heavy-loss encoder is lower than 60\%, the central controller tries to compress the upstream and downstream heavy-loss encoders to approach 75\% load factor.
%
Note that the upstream and downstream flow encoders can be compressed up to their reserved memory, \ie, $m_{hl}$ is at least set to $m^{res}_{hl}$.
%
If they are compressed to their reserved memory, the network condition transitions to the green network condition.
%
\subsubsection{Red network condition:}
\label{sec:red}
Under red network condition, there is a fixed memory configuration that $m_{hh}$, $m_{hl}$ and $m_{ll}$ are set to $m^{hh}_{res}$, $m^{uf} - m^{hh}_{res} - m^{ll}_{res}$, and $m^{ll}_{res}$, respectively;
%
\ykc{For each edge switch, the threshold $T_h$ can be set to an arbitrary value, while $T_l$ and the sampling rate must be unified.}
%
Suppose the network condition sensed in the last round of self-adaptation is red, and now the central controller starts the next round.

\bbb{Sensing real-time network condition:}
The central controller first estimates the number of flows, the number of heavy-hitter candidates, and the flow size distribution of each edge switch in a similar way to that in green network condition.
%
In addition, the central controller obtains the number of light-losses before sampling by decoding the delta light-loss encoder as described in packet loss detection ($\S$~\ref{tasks:flow}).
%
If both the decoding of the delta heavy-loss and light-loss encoders succeeds, the central controller estimates the number and flow size distribution of victim flows as follows.
%
First, the central controller samples the heavy-losses with the same sampling method and rate as light-losses.
%
Second, the central controller merges the sampled heavy-losses and sampled light-losses to obtain the sampled victim flows.
%
Third, the central controller estimates the flow size distribution of victim flows through querying the flow sizes of sampled victim flows, and the number of victim flows through dividing the number of sampled victim flows by the sampling rate.
%
Otherwise, the central controller simply approximates the flow size distribution of victim flows with the estimated flow size distribution of sampled light-losses.
%
\ykc{The accuracy of the approximation gradually improves as the threshold $T_l$ increases.}

\bbb{Reconfiguring memory and thresholds:}
First, if the decoding of any upstream heavy-hitter encoder fails, the central controller first turns down the threshold $T_h$ to control the expected load factor of the upstream heavy-hitter encoder at around 75\%, and then terminates this round of the self-adaptation.
%
%
%Otherwise, if the decoding of the delta light-loss encoder fails, the central controller simply sets the  threshold $T_l$ is to $T_h$ and then stops the self-adaptation.
%
%

Second, if the decoding of the delta light-loss encoder fails, according to the estimated number of light-losses, the central controller reconfigures the sampling rate to control the expected load factor of the delta light-loss encoder at around 75\% and then stops the self-adaptation, and then terminates this round of the self-adaptation.
%

Third, if the decoding of the delta heavy-loss encoder fails, according to the estimated flow size distribution of victim flows, the central controller turns up the threshold $T_l$ to control the expected load factor of the delta heavy-loss encoder at around 75\%.
%
%

Fourth, if all the decoding succeeds, according to the estimated number of victim flows, the central controller estimates the required memory for recording all the victim flows with a load factor around 75\%.
%
If the downstream flow encoder can cover the required memory, the central controller then 1) eliminates the light-loss encoders, 2) configures the heavy-loss encoders with the required memory, and 3) sets the threshold $T_l$ to 0.  
%
In this case, the red network condition transitions back to yellow or green network condition.
%
Otherwise, if the load factor of the delta heavy-loss encoder or the delta light-loss encoder is lower than 60\%, the central controller reconfigures $T_l$ or the sampling rate based on the estimated flow size distribution of victim flows or the estimated number of light-losses before sampling, respectively.

After all the memory reconfigurations, for each edge switch, the central controller also turns down or up the threshold $T_h$ of the edge switch to control the load factor of its upstream heavy-hitter encoder between 60\% and 70\%.


% \bbb{Analyzing real-time network condition:}
% At the beginning, we need to analyze the real-time network condition to estimate the number of potential heavy-hitters, heavy-losses, and light-losses in the last measurement window, so as to further estimate the memory overhead required to record them in the next window.
% %
% To achieve this, we first estimate the numbers of potential heavy-hitters of each switch.
% %
% We decode the upstream heavy-hitter encoders collected from every edge switch individually.
% %
% For any edge switch, if the decoding of its heavy-hitter encoder succeeds, we can directly obtain its number of potential heavy-hitters.
% %
% Otherwise, we apply linear-counting algorithm \cite{whang1990linear} to any of the arrays of its heavy-hitter encoder to obtain its number of potential heavy-hitters.
% %
% Considering that the heavy-hitter encoder must be the same size on every edge switch, we take the maximum value of the numbers of potential heavy-hitters of all switches for further estimating the memory overhead required to record them.
% %
% Second, we estimate the number of potential heavy-losses in the network.
% %
% For every edge switch, we reinsert all its decoded potential heavy-hitters into its upstream heavy-loss encoder.
% %
% Then, We adding up all the upstream/downstream heavy-loss encoders to obtain a cumulative upstream/downstream heavy-loss encoder, and then subtract the downstream one from the upstream one.
% %
% Next, we decode the upstream heavy-loss encoder and estimate the number of potential heavy-losses in the network in a similar way to estimating the number of potential heavy-hitters.
% %
% \ykc{Note that we do not estimate the number of potential heavy-losses if the decoding of any of the upstream heavy-hitter encoders fails.}
% %
% Third, we estimate the number of potential light-losses in the network in a similar way to estimating the number of heavy-losses, except we do not reinsert potential heavy-hitters into the upstream light-loss encoders.
% %


% \bbb{Generating and applying appropriate memory reconfiguration schemes:}
% With the estimated number of potential heavy-hitters, heavy-losses, and light-losses, we can then estimate the minimum memory overhead required to record them, generate appropriate memory reconfiguration schemes under the given memory constraint, and apply the generated schemes to switch data planes.
% %
% %
% At a high level, the memory configuration has two modes: 1) the light-loss encoder is not allocated any memory and the threshold $\mathcal{T}_l$ for identifying heavy-losses is set to $0$; 2) the light-loss encoder is allocated a certain amount of memory and $\mathcal{T}_l$ is set to \ykc{a user-defined value}.
% %
% The first mode applies to the network condition where the given memory is enough for recording all the potential heavy-hitters and victim flows, and the second mode applies to the network condition where the given memory is not enough for recording all the potential heavy-hitters and victim flows, and thus aim at recording all the heavy-hitters and heavy-losses, and a portion of light-losses through sampling.
% %
% %
% %

% Then, we detail how to generate appropriate memory reconfiguration schemes with the estimated number of heavy-hitters, heavy-losses, and light-losses.
% %
% Here, we assume that the upstream flow encoder always has enough memory to record all the heavy-hitters.
% %
% Suppose the upstream flow encoder and the downstream flow encoder consist of $d$ bucket arrays, and the numbers of buckets per array are $m_{uf}$ and $m_{df}$, respectively.
% %
% %
% At initialization, the configuration is in the first mode: parameters $m_{hh}$, $m_{hl}$, $m_{ll}$ are set to $(m_{uf}-m_{df})$, $m_{df}$, $0$, respectively; Threshold $T_h$ is set to a user-defined value and $T_l$ is set to $0$.
% %
% We first propose how to reconfigure the memory if the current configuration is in the first mode.
% %
% Every time after we analyze the network condition in the last measurement window, we first estimate the minimum values for $m_{hh}$ and $m_{hl}$ required to record the estimated numbers of potential heavy-hitter and heavy-losses, denoted by $m^{e}_{hh}$ and $m^{e}_{hl}$, respectively. 
% %
% The estimation method is similar to that of IBLT \cite{goodrich2011invertibleIBLT}, that we can multiplying the number of flows by a coefficient corresponding to the number of arrays $d$ (\eg, $1.22$ when $d=3$) to obtain the minimum number of buckets to record these flows.
% %
% %
% if both of the decoding of potential heavy-hitters and heavy-losses succeed, we do not generate any scheme.
% %  
% If the decoding of potential heavy-hitters fails, we set $m_{hh}$ to $p \times m^{e}_{hh}$ and $m_{hl}$ to $m_{uf} - p \times m^{e}_{hh}$, where $p > 1$.
% %
% Here, we allocate $p$ times minimum required memory to the upstream heavy-hitter encoder for two reasons: 1) the measurement and reconfiguration inevitably has a lag, and the extra memory is to cope with the potential increment of potential heavy-hitters during the lag; 2) the estimated number of heavy-hitters is inaccurate when the decoding fails, and we allocate more memory to tolerate the error. 
% %
% Also, such allocation applies to the heavy-loss and light-loss encoders. 
% %
% If the decoding of potential heavy-losses fails, there are two branches:
% %
% If it satisfies that $p \times m^{e}_{hl} \leq m_{df}$ and $p \times (m^{e}_{hh} + m^{e}_{hl}) \leq m_{uf}$, we consider that the flow encoders can record all the potential heavy-hitters and heavy-losses: we set $m_{hh}$ to $m_{uf} - p \times m^{e}_{hl}$ and $m_{hl}$ to $p \times m^{e}_{hl}$;
% %
% Otherwise, we switch the configuration to the second mode.
% %

% %
% In the second mode, at initialization, we first set $T_l$ to a user-defined value for distinguishing between potential heavy-losses and light-losses.
% %
% Considering that we have no information about the number of potential heavy-losses, we just compress the upstream/downstream heavy-loss encoders to half their sizes, while the memory saved is allocated to the upstream/downstream light-loss encoders, and the sampling rate of light-losses, denoted by $R$, is set to $1$.
% %
% Then, we propose how to reconfigure the memory if the current configuration is in the second mode.
% %
% Every time after we analyze the network condition in the last measurement window, we estimate $m^{e}_{hh}$, $m^{e}_{hl}$, and the minimum value for $m_{ll}$ required to record all the potential light-losses before sampling, denoted by $m^{e}_{ll}$. 
% %
% %
% First, we check whether the decoding of heavy-hitters succeeds.
% %
% If succeeds, we check whether $m_{hh} > p \times m^{e}_{hh}$.
% %
% If so, we compress $m_{hh}$ to $MIN(p \times m^{e}_{hh}, m_{uf} - m_{df})$, and the store saved memory in a memory pool.
% %
% If fails, the upstream heavy-hitter encoder first steals memory from the light-loss encoder, and then the heavy-loss encoder, so as to set $m_{hh}$ to $p \times m^{e}_{hh}$.
% %
% %
% Second, we check whether the decoding of heavy-losses succeeds.
% %
% If succeeds, we check whether $m_{hl} > p \times m^{e}_{hl}$.
% %
% If so, we compress $m_{hl}$ to $p \times m^{e}_{hh}$, and the saved memory are stored in the memory pool.
% %
% If fails, the upstream/downstream heavy-loss encoder first steals memory from the memory pool, and then the light-loss encoder, so as to set $m_{hl}$ to $p \times m^{e}_{hl}$.
% %
% Third, the upstream/downstream light-loss encoder steals all the memory in the memory pool, and the sampling rate $R$ is set to $MAX(1, \frac{m_{ll}}{p \times m^{e}_{ll}})$.
% %
% Finally, if $R$ is set to $1$, we merge the light-loss encoders to the heavy-loss encoders, set $T_l$ to $0$, and switch the configuration to the first mode.
% %
% Then, the generated configuration schemes are forwarded to the control plane of each edge switch, and applied to the switch data plane to function in the next measurement window. 
